# Supplementary material for: SpaRP: Fast 3D Object Reconstruction and Pose Estimation from Sparse Views
Source: arXiv:2408.10195 source file (2024-08-19)
Supplement: Supplementary file 1 [file supp_mixed.tex]

\begin{table}[b]
  \caption{\textbf{Effect of Joint Training.} Evaluated on 500 objects from the Google Scanned Objects (GSO) dataset~\cite{downs2022google}.}
  \centering

  \begin{tabular}{c|c|cc}
    \toprule

    \multicolumn{2}{c}{Metrics} & Separate Training & Joint Training \\
    \midrule
    \multirow{4}{*}{\makecell{Pose \\ Estimation}} 
    & Rotation Error $\downarrow$ & 9.87 & \textbf{8.57} \\
    & Accuracy@15$^{\circ}\uparrow$ & 0.563 & \textbf{0.601} \\
    & Accuracy@30$^{\circ}\uparrow$ & 0.617 & \textbf{0.677} \\
    & Translation Error $\downarrow$ & 0.42 & \textbf{0.37} \\
    \hline
    \multirow{4}{*}{\makecell{3D \\ Reconstruction}} 
    & F-Score $\uparrow$ & 96.81 & \textbf{97.12} \\
    & CLIP-Similarity $\uparrow$ & 78.36 & \textbf{78.90} \\
    & PSNR $\uparrow$ & 19.03 & \textbf{19.42} \\
    & LPIPS $\downarrow$ & 0.129  & \textbf{0.128}  \\
    
    \bottomrule
  \end{tabular}
  \label{tab:mixed}
\end{table}
